# Supplementary material for: Effects of Modal Dispersion on Few Photon - Qubit Scattering in One-Dimensional Waveguides
Source: arXiv:1510.03069 ancillary file (2016-03-14)

```

x = x; Remove["Global`*"];
Off[General::spell];
Off[General::spell1];
<< "AuthorTools`"
SetDirectory[NotebookFolder[EvaluationNotebook[]]];

```

## Definitions

---

These are common definitions used throughout the paper and used in the generation of figures. Equation numbers from the paper are given as comments.

```

J = 1;
(* General form of I(z) integral in eqn (A1) for complex z *)
Int[z_?NumericQ] := Block[{v1 = ArcCos[- $\frac{zb}{2}$ ], J = 1},
  If[Im[v1] < 0, v1 = -v1];
  
$$\frac{2\pi i}{-2J \sin[v1]}$$
 // N
];
(* Eqn (26) *)
H[z_,  $\Omega$ _, g_, wp_] := z -  $\Omega$  - wp - g2 Int[z - wp];
(* This is the V0 approximation for U, given in eqn (42) *)
U0[z_?NumericQ,  $\Omega$ _?NumericQ, g_?NumericQ, wp_?NumericQ, wk_?NumericQ] :=  $\frac{1}{z - wp - wk}$ ;
(* This is the V0 + V1 approximation for U, with V1 given in eqn (43) *)
U1[z_?NumericQ,  $\Omega$ _?NumericQ, g_?NumericQ, wp_?NumericQ, wk_?NumericQ] :=

$$\frac{1}{z - wp - wk} + g^2 \text{NIntegrate}\left[\frac{1}{z - wp + 2 * J * \cos[v]} \frac{1}{H[z, \Omega, g, -2 * J * \cos[v]]}\right.$$


$$\left. \frac{1}{z - wk + 2 * J * \cos[v]}, \{v, -\pi, \pi\}, \text{PrecisionGoal} \rightarrow 3, \text{MaxRecursion} \rightarrow 1000, \right.$$


$$\left. \text{Method} \rightarrow \{\text{GlobalAdaptive}, \text{MaxErrorIncreases} \rightarrow 10\,000\} \right];$$

(* This is the V0 + V1 + V2 approximation for U, with V2 given in eqn (44) *)
U2[z_?NumericQ,  $\Omega$ _?NumericQ, g_?NumericQ, wp_?NumericQ, wk_?NumericQ] :=

$$\frac{1}{z - wp - wk} + g^2 \text{NIntegrate}\left[\frac{1}{z - wp + 2 * J * \cos[v]} \frac{1}{H[z, \Omega, g, -2 * J * \cos[v]]}\right.$$


$$\left. \frac{1}{z - wk + 2 * J * \cos[v]}, \{v, -\pi, \pi\}, \text{PrecisionGoal} \rightarrow 3, \text{MaxRecursion} \rightarrow 1000, \right.$$


$$\left. \text{Method} \rightarrow \{\text{GlobalAdaptive}, \text{MaxErrorIncreases} \rightarrow 10\,000\} \right] + g^4 \text{NIntegrate}\left[\right.$$


$$\frac{1}{z - wp + 2 * J * \cos[v2]} \frac{1}{H[z, \Omega, g, -2 * J * \cos[v2]]} \frac{1}{z + 2 * J * \cos[v2] + 2 * J * \cos[v1]}$$


$$\left. \frac{1}{H[z, \Omega, g, -2 * J * \cos[v1]]} \frac{1}{z + 2 * J * \cos[v1] - wk}, \{v1, -\pi, \pi\}, \{v2, -\pi, \pi\}, \right.$$


$$\left. \text{PrecisionGoal} \rightarrow 3, \text{MaxRecursion} \rightarrow 1000, \text{Method} \rightarrow \{\text{GlobalAdaptive}, \right.$$


$$\left. \text{Method} \rightarrow \text{"GaussBerntsenEspelidRule"}, \text{MaxErrorIncreases} \rightarrow 100\,000\} \right];$$

(* This is the B function from the last line in (46) without the Dirac delta term. TB stands for tight-binding. *)
BTB[en_,  $\Omega$ _, g_, order_,  $\Delta E_k$ _,  $\Delta E_p$ _] :=
Module[{wk1 =  $\frac{en}{2} + \Delta E_k$ , wk2 =  $\frac{en}{2} - \Delta E_k$ , wp1 =  $\frac{en}{2} + \Delta E_p$ , wp2 =  $\frac{en}{2} - \Delta E_p$ ,
  Ux = Which[order == 0, U0, order == 1, U1, order == 2, U2, True, Throw["Wrong order"]]},

```

```

-2 π i * g^4 * (
  (Ux[en, Ω, g, wp1, wk1] / (H[en, Ω, g, wp1] H[en, Ω, g, wk1]) +
  Ux[en, Ω, g, wp1, wk2] / (H[en, Ω, g, wp1] H[en, Ω, g, wk2]) +
  Ux[en, Ω, g, wp2, wk1] / (H[en, Ω, g, wp2] H[en, Ω, g, wk1]) +
  Ux[en, Ω, g, wp2, wk2] / (H[en, Ω, g, wp2] H[en, Ω, g, wk2])
)
];

(* This is the production amplitude for free to bound scattering,
used as the T function, defined in eqn (39) without the Dirac delta term *)
ProdTB[g_, η_, wpm_, pb_, wk1_, wk2_] := Module[{zos, Ek},
  zos = wk1 + wk2;
  (-2 π i) √pb * g^3 *
  (
    (U1[zos + i * η, 0, g, wk1 + wk2 - wpm, wk1] /
     H[zos, 0, g, wk1]) +
    (U1[zos + i * η, 0, g, wk1 + wk2 - wpm, wk2] /
     H[zos, 0, g, wk2])
  )
];

(* Normalized 1-photon Gaussian in k-space,
Fourier transformed version of the one presented in Sec VI *)
fkGauss[k_, xc_, s_, k0_] := 1 / (π * 1 / s^2)^{1/4} * Exp[-(k - k0)^2 / (2 * 1 / s^2) - i * (k - k0) * xc];

(* Normalized 2-
photon Gaussian packet with the same center k0 value for the two photons *)
fk2Gauss[k1_, k2_, xc_, s_, k0_] := fkGauss[k1, xc, s, k0] * fkGauss[k2, xc, s, k0];
(* 1-photon reflection coefficient from eqn (19) *)
r1[J_, gp_, Ω_, k_] := -gp^2 / (2 i * J * Abs[Sin[k]] (Ω + 2 J * Cos[k]) + gp^2);
(* 1-photon transmission coefficient from eqn (20) *)
t1[J_, gp_, Ω_, k_] := 1 + (-gp^2) / (2 i * J * Abs[Sin[k]] (Ω + 2 J * Cos[k]) + gp^2);
(* Implementation of eqn (51) *)
FreetoFreeTB[p1_?NumericQ, p2_?NumericQ, Ω_?NumericQ,
g_?NumericQ, xc_?NumericQ, s_?NumericQ, k0_?NumericQ] := Module[
{wp1 = -2 J * Cos[p1], wp2 = -2 J * Cos[p2], zpos = -2 J * Cos[p1] - 2 J * Cos[p2], J = 1},
fk2Gauss[p1, p2, xc, s, k0] * t1[J, √(2 π) g, Ω, p1] * t1[J, √(2 π) g, Ω, p2] +
fk2Gauss[-p1, -p2, xc, s, k0] * r1[J, √(2 π) g, Ω, p1] * r1[J, √(2 π) g, Ω, p2] +
fk2Gauss[p1, -p2, xc, s, k0] * t1[J, √(2 π) g, Ω, p1] * r1[J, √(2 π) g, Ω, p2] +
fk2Gauss[-p1, p2, xc, s, k0] * r1[J, √(2 π) g, Ω, p1] * t1[J, √(2 π) g, Ω, p2] +
1/2 NIntegrate[
  (fk2Gauss[ArcCos[(zpos/2 + ΔEk)/(-2 J)], ArcCos[(zpos/2 - ΔEk)/(-2 J)], xc, s, k0) +
  fk2Gauss[-ArcCos[(zpos/2 + ΔEk)/(-2 J)], ArcCos[(zpos/2 - ΔEk)/(-2 J)], xc, s, k0) +
  fk2Gauss[-ArcCos[(zpos/2 + ΔEk)/(-2 J)], -ArcCos[(zpos/2 - ΔEk)/(-2 J)], xc, s, k0) +
  fk2Gauss[ArcCos[(zpos/2 + ΔEk)/(-2 J)], -ArcCos[(zpos/2 - ΔEk)/(-2 J)], xc, s, k0)
] *

```

```

BTB[zpos, Ω, g, 0, ΔEk,  $\frac{wp1 - wp2}{2}$ ] *  $\frac{1}{\sqrt{4 * J^2 - (\frac{zpos}{2} + \Delta Ek)^2}}$  *  $\frac{1}{\sqrt{4 * J^2 - (\frac{zpos}{2} - \Delta Ek)^2}}$ ,
{ΔEk, Max[-2 +  $\frac{wp1 + wp2}{2}$ , -2 -  $\frac{wp1 + wp2}{2}$ ], Min[2 -  $\frac{wp1 + wp2}{2}$ , 2 +  $\frac{wp1 + wp2}{2}$ ]}},
PrecisionGoal → 4]]];

(* Implementation of eqn (50) *)
FreeToBoundTB[p_?NumericQ, wpm_?NumericQ, Ω_ /; Ω == 0,
g_?NumericQ, η_?NumericQ, xc_?NumericQ, s_?NumericQ, k0_?NumericQ] :=
Module[{wp = -2 J * Cos[p], zpos, J = 1, pb},
zpos = wp + wpm;
pb =  $\frac{(2 \pi)^2 g^4}{2 * wp^2 * (wp^2 - 2 * J^2)}$ ;
NIntegrate[ $\left( \text{fk2Gauss}\left[\text{ArcCos}\left[\frac{(\frac{zpos}{2} + \Delta Ek)}{(-2 J)}\right], \text{ArcCos}\left[\frac{(\frac{zpos}{2} - \Delta Ek)}{(-2 J)}\right], xc, s, k0\right] + \right.$ 
fk2Gauss[ $-\text{ArcCos}\left[\frac{(\frac{zpos}{2} + \Delta Ek)}{(-2 J)}\right], \text{ArcCos}\left[\frac{(\frac{zpos}{2} - \Delta Ek)}{(-2 J)}\right], xc, s, k0\right] +$ 
fk2Gauss[ $-\text{ArcCos}\left[\frac{(\frac{zpos}{2} + \Delta Ek)}{(-2 J)}\right], -\text{ArcCos}\left[\frac{(\frac{zpos}{2} - \Delta Ek)}{(-2 J)}\right], xc, s, k0\right] +$ 
fk2Gauss[ $\text{ArcCos}\left[\frac{(\frac{zpos}{2} + \Delta Ek)}{(-2 J)}\right], -\text{ArcCos}\left[\frac{(\frac{zpos}{2} - \Delta Ek)}{(-2 J)}\right], xc, s, k0\right] \left. \right) *$ 
ProdTBManual[g, η, wpm, pb,  $\frac{zpos}{2} + \Delta Ek, \frac{zpos}{2} - \Delta Ek$ ] *
 $\frac{1}{\sqrt{4 * J^2 - (\frac{zpos}{2} + \Delta Ek)^2}}$  *  $\frac{1}{\sqrt{4 * J^2 - (\frac{zpos}{2} - \Delta Ek)^2}}$ ,
{ΔEk, Max[-2 +  $\frac{zpos}{2}$ , -2 -  $\frac{zpos}{2}$ ], Min[2 -  $\frac{zpos}{2}$ , 2 +  $\frac{zpos}{2}$ ]}}, PrecisionGoal → 4]]];

```

**Fig 1**

Here, we solve for the polynomial equation for the bound modes, and weed out unphysical roots.

```

Block[{f, ftest, fpoly, gp, OmegaList, resultList, soln},
f[z_, Ω_, gp_] := Piecewise[{{z - Ω - gp^2 / Sqrt[(z)^2 - 4], z > 2},
{z - Ω + gp^2 / Sqrt[(z)^2 - 4], z < -2}, {z - Ω + I gp^2 / Sqrt[4 - z^2], -2 < z < 2}}];
ftest[z_, Ω_, gp_] := z - Ω - gp^2 / (2 π) Int[z];
fpoly[z_, Ω_, gp_] := (z^2 - 4) (z - Ω)^2 - gp^4;
gp = 1.0;
OmegaList = Table[Ω, {Ω, -5.0, 5.0, 0.05}];
resultList = {};
For[i = 1, i ≤ Length[OmegaList], i++,
soln = Cases[z /. NSolve[fpoly[z, OmegaList[[i]], gp] == 0], _Real];
For[j = 1, j ≤ Length[soln], j++,
If[Abs[ftest[soln[[j]], OmegaList[[i]], gp]] < 10^-5,
AppendTo[resultList, {OmegaList[[i]], soln[[j]]}];
];
];
p1 = ListPlot[{Select[resultList, #[[2]] > 0 &], Select[resultList, #[[2]] < 0 &]},
Joined → True, PlotStyle → {Blue, Black}, AxesLabel → {"Ω", "ω±"},
Epilog → {Dashed, Red, Line[{{5, 5}, {-5, -5}}]},
Ticks → {Range[-5, 5, 1], Range[-5, 5, 1]}, ImageSize → 72 * 3.4];
Export["./fig01/fig01_boundStateMinusData_g" <> ToString[IntegerPart[10 * gp]] <> ".tsv",
Select[resultList, #[[2]] < 0 &]];
Export["./fig01/fig01_boundStatePlusData_g" <> ToString[IntegerPart[10 * gp]] <> ".tsv",
Select[resultList, #[[2]] > 0 &]];
];
Show[p1]
Clear[p1]

```

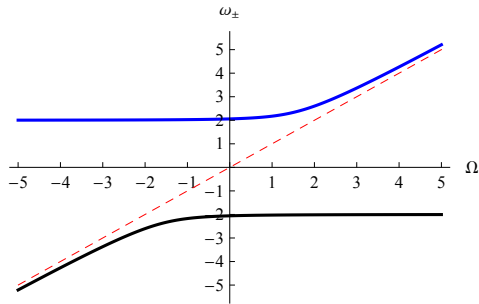
**Fig 2**

This figure examines the properties of the bound state for  $\Omega=0$ , given in App. B.

```

Block[{gp, wp, pb, x, Bplus, Bminus},
  gp = 1;
  wp =  $\sqrt{2 * J^2 + \sqrt{4 * J^4 + gp^4}}$ ;
  pb =  $gp^4 / (2 * wp^2 * (wp^2 - 2 * J^2))$ ;
  Bplus =
    Table[{x, gp *  $\sqrt{pb}$  *  $\left(-wp / (2 * J) + \sqrt{(wp^2 / (4 * J^2) - 1)}\right)^{Abs[x]} / \sqrt{wp^2 - 4 * J^2}}$ ,
      {x, -30, 30}];
  Bminus = Table[{x, gp *  $\sqrt{pb}$  *  $(-1) * \left(wp / (2 * J) - \sqrt{(wp^2 / (4 * J^2) - 1)}\right)^{Abs[x]} / \sqrt{wp^2 - 4 * J^2}}$ ,
    {x, -30, 30}];
  p1 = ListPlot[{Bplus, Bminus}, Filling -> Axis, PlotRange -> All, Frame -> True];
  Export["./fig02/fig02_BoundStateSpace_g" <> ToString[IntegerPart[10 * gp]] <> ".tsv",
    Transpose[N[{Bminus[[;;, 1]], Bminus[[;;, 2]], Bplus[[;;, 2]]}]]];
];
Show[p1]
Clear[p1]

```

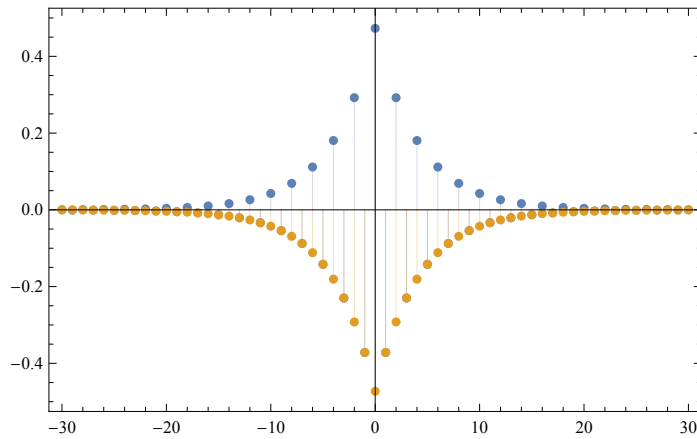

**Fig 3**

Implementation of equations (C1) and (C2) that gives  $e(t)$ .

```

Block[{gp, wp, pb, exactTest, resultList},
  gp = 2;
  wp =  $\sqrt{2 * J^2 + \sqrt{4 * J^4 + gp^4}}$ ;
  pb = gp^4 / (2 * wp^2 * (wp^2 - 2 * J^2));
  exactTest[g_, t_] := Module[{s1 = Sqrt[Sqrt[4 + g^4] - 2], s3 = Sqrt[Sqrt[4 + g^4] + 2]},
    2 * (1 / 4 + 2 / (4 Sqrt[4 + g^4])) Cosh[s1 * t] +
    2 * (1 / 4 - 2 / (4 Sqrt[4 + g^4])) Cos[s3 * t] - 2 * (g^2 / (4 Sqrt[4 + g^4]))
    (NIntegrate[(s3^2 / s1 Sinh[s1 * (t - u)] + s1^2 / s3 Sin[s3 * (t - u)])
      BesselJ[0, 2 * u], {u, 0, t}, WorkingPrecision -> 50])
  ];
  resultList = Table[{t, Abs[exactTest[gp, t]]^2}, {t, 0, 30, 1 / 10}];
  p1 = ListPlot[resultList, PlotRange -> {0, 1}, Joined -> True,
    AxesLabel -> {"t", "e(t)"}, ImageSize -> 72 * 3.4, PlotLabel -> "g'=" <> ToString[gp],
    PlotMarkers -> Graphics@{Disk[{0, 0}, Scaled@0.008]},
    Epilog -> {Dashed, Line[{0, 4 * pb^2}, {50, 4 * pb^2}]}];
  Export["./fig03/fig03_boundStateTimeEvolutionData_g" <>
    ToString[IntegerPart[10 * gp]] <> ".tsv", N[resultList, 10]];
];
Show[p1]
Clear[p1]

```

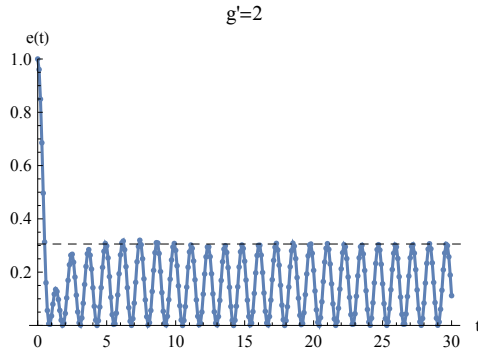

**Fig 7**

### ■ Calculate Feynman Integrals

The block below calculates Feynman integrals using U0, U1 and U2 functions as we sweep k0 to get different approximations to the bound to bound reflection coefficient in eqn (37). U2 calculations take some time.

```

Block[{gplist, kList, r0list, r1list, r2list, dum,
  temp, gp, J, xc, s, wplus, pb, g, k, z, result0, result1, result2},
  gplist = {0.5, 1.0};
  kList = Table[k, {k,  $\pi/6$ ,  $5\pi/6$ ,  $\pi/60$ ]];
  dum = TimeUsed[];
  Print[DateString["Time"]];
  temp = PrintTemporary["Starting evaluation... "];
  For[j = 1, j ≤ Length[gplist], j++,
    gp = gplist[[j]];
    J = 1; xc = 0; s = 12;
    
$$g = \frac{gp}{\sqrt{2\pi}};$$

    
$$wplus = \sqrt{2 * J^2 + \sqrt{4 * J^4 + gp^4}};$$

    
$$pb = \frac{gp^4}{2 * wplus^2 * (wplus^2 - 2 * J^2)};$$

    r0list = ConstantArray[{0.0, 0.0, 0.0, 0.0}, Length[kList]];
    r1list = ConstantArray[{0.0, 0.0, 0.0, 0.0}, Length[kList]];
    r2list = ConstantArray[{0.0, 0.0, 0.0, 0.0}, Length[kList]];
    For[i = 1, i ≤ Length[kList], i++,
      k = kList[[i]];
      (* Calculate for (-) bound state *)
      z = -2 J * Cos[k] - wplus;
      result0 = U0[z + i * 10-6, 0, g, -2 J * Cos[k], -2 J * Cos[k]];
      result1 = U1[z + i * 10-6, 0, g, -2 J * Cos[k], -2 J * Cos[k]];
      result2 = U2[z + i * 10-4, 0, g, -2 J * Cos[k], -2 J * Cos[k]];
      r0list[[i]] = {g, k, -2 *  $\pi$  * i * pb * g2 *  $\frac{result0}{2 * J * Abs[Sin[k]]}}$  // N;
      r1list[[i]] = {g, k, -2 *  $\pi$  * i * pb * g2 *  $\frac{result1}{2 * J * Abs[Sin[k]]}}$  // N;
      r2list[[i]] = {g, k, -2 *  $\pi$  * i * pb * g2 *  $\frac{result2}{2 * J * Abs[Sin[k]]}}$  // N;
    Export[
      "./fig07/integrals_r0_g" <> ToString[IntegerPart[10 * gp]] <> ".tsv", r0list];
    Export["./fig07/integrals_r1_g" <> ToString[IntegerPart[10 * gp]] <> ".tsv",
      r1list];
    Export["./fig07/integrals_r2_g" <> ToString[IntegerPart[10 * gp]] <> ".tsv",
      r2list];

    NotebookDelete[temp];
    temp =
      PrintTemporary[ToString[TimeUsed[] - dum] <> " seconds for i=" <> ToString[i] <>
        " of " <> ToString[Length[kList] * Length[gplist]] <> ". Total time estimate " <>
        ToString[(TimeUsed[] - dum) / i * (Length[kList] * Length[gplist])] <> " sec."];
  ];
];
Print[ToString[TimeUsed[] - dum] <> " seconds total - " <> DateString["Time"]];
];

```

```
16:51:19
```

```
11152.3 seconds total - 19:57:16
```

### ■ Interpolation and Gaussian Integration

This block implements the gaussian integration in eqn (47). But first, it fits an interpolation function to the previously obtained results to speed up calculations.



```

Block[{xc, s, gp, r0list, r1list, r2list, R0list, R1list, R2list, T0list,
  T1list, T2list, funR1, funR2, funT1, funT2, intResults, k0, R1, T1, R2, T2},
  xc = 0; s = 12;
  gp = 1;
  r0list = ToExpression[
    Import["./fig07/integrals_r0_g" <> ToString[IntegerPart[10 * gp]] <> ".tsv"]];
  r1list = ToExpression[Import["./fig07/integrals_r1_g" <>
    ToString[IntegerPart[10 * gp]] <> ".tsv"]];
  r2list = ToExpression[Import["./fig07/integrals_r2_g" <>
    ToString[IntegerPart[10 * gp]] <> ".tsv"]];
  R0list = ({#[[2]], Abs[#[[3]]]^2}) & /@ r0list;
  R1list = ({#[[2]], Abs[#[[3]]]^2}) & /@ r1list;
  R2list = ({#[[2]], Abs[#[[3]]]^2}) & /@ r2list;
  T0list = ({#[[2]], Abs[1 + #[[3]]]^2}) & /@ r0list;
  T1list = ({#[[2]], Abs[1 + #[[3]]]^2}) & /@ r1list;
  T2list = ({#[[2]], Abs[1 + #[[3]]]^2}) & /@ r2list;
  funR1 = Interpolation[R1list];
  funR2 = Interpolation[R2list];
  funT1 = Interpolation[T1list];
  funT2 = Interpolation[T2list];

  (* Calculate gaussian integrals *)
  intResults = {};
  For[i = 1, i ≤ Length[r1list], i++,
    k0 = r1list[[i, 2]];
    R1 = NIntegrate[funR1[kk] * Abs[fkGauss[kk, xc, s, k0]]^2,
      {kk, k0 - π, k0 + π}, PrecisionGoal → 7];
    T1 = NIntegrate[funT1[kk] * Abs[fkGauss[kk, xc, s, k0]]^2,
      {kk, k0 - π, k0 + π}, PrecisionGoal → 7];
    R2 = NIntegrate[funR2[kk] * Abs[fkGauss[kk, xc, s, k0]]^2,
      {kk, k0 - π, k0 + π}, PrecisionGoal → 7];
    T2 = NIntegrate[funT2[kk] * Abs[fkGauss[kk, xc, s, k0]]^2,
      {kk, k0 - π, k0 + π}, PrecisionGoal → 7];
    AppendTo[intResults, {k0, R1, T1, 1 - R1 - T1, R2, T2, 1 - R2 - T2}];
  ];

  (* Visualize *)
  Print[ListPlot[{intResults[[;;, 1;; 2;; 1]], intResults[[;;, 1;; 3;; 2]],
    intResults[[;;, 1;; 4;; 3]], intResults[[;;, 1;; 5;; 4]],
    intResults[[;;, 1;; 6;; 5]], intResults[[;;, 1;; 7;; 6]]},
    PlotStyle → {{Dashed, Opacity[0.5], Blue}, {Dashed, Opacity[0.3], Black},
      {Dashed, Opacity[0.3], Red}, Blue, Black, Red},
    PlotLabel → "R(Blue) T(Black) 1-R-T(Red)", PlotRange -> All, Joined → True,
    PlotMarkers → Graphics@{Disk[{0, 0}, Scaled@0.02]}]];

  (* Save data *)
  Export["./fig07/fig07_integrals_Gaussian_g" <>
    ToString[IntegerPart[10 * gp]] <> ".tsv", intResults];
];

```

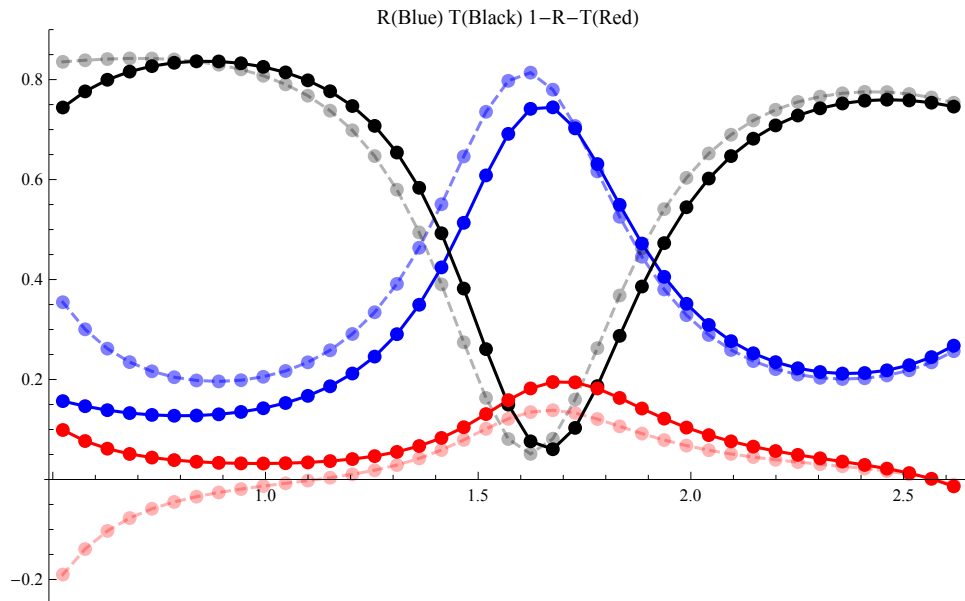**Fig 9**

This block implements the p-integrals in eqn (50) in calculating  $\langle \text{out} | \text{out} \rangle$ .

```
Block[{η, g, J, gp, wplus, pb, enDiscrete, ProdTBpluslist, ProdTBminuslist,
  dum, temp, ProdTBplotlist, ProdTBplotlistfiltered, jet, ProdTBPlot, img,
  ProdTBplusInterp, ProdTBminusInterp, xc, s, kList, resultList, i1, i2},
  η = 10-6; g = 0.5 /  $\sqrt{2\pi}$  // N; J = 1;
  gp = g *  $\sqrt{2\pi}$ ;
  wplus =  $\sqrt{2 * J^2 + \sqrt{4 * J^4 + gp^4}}$ ;
  pb =  $\frac{gp^4}{2 * wplus^2 * (wplus^2 - 2 * J^2)}$ ;
  enDiscrete = Range[-2, 2, 0.05];

  (* Create the data for subplot (a) *)
  ProdTBpluslist =
    ConstantArray[{0.0, 0.0, 0.0}, {Length[enDiscrete], Length[enDiscrete]}];
  ProdTBminuslist = ConstantArray[{0.0, 0.0, 0.0},
    {Length[enDiscrete], Length[enDiscrete]}];
  dum = TimeUsed[];
  temp = PrintTemporary["Starting evaluation..."];
  For[ii = 1, ii ≤ Length[enDiscrete], ii++,
    For[jj = 1, jj ≤ Length[enDiscrete], jj++,
      ProdTBpluslist[[ii, jj]] = {enDiscrete[[ii]], enDiscrete[[jj]],
        ProdTB[g, η, wplus, pb, enDiscrete[[ii]], enDiscrete[[jj]]]};
      ProdTBminuslist[[ii, jj]] = {enDiscrete[[ii]], enDiscrete[[jj]],
        ProdTB[g, η, -wplus, pb, enDiscrete[[ii]], enDiscrete[[jj]]]};
    ];
  NotebookDelete[temp];
  temp = PrintTemporary["Subplot (a): " <> ToString[TimeUsed[] - dum] <>
    " seconds for ii=" <> ToString[ii] <> " of " <> ToString[Length[enDiscrete]]];
];
Print[ToString[TimeUsed[] - dum] <> " seconds total for " <>
```

```

ToString[Length[enDiscrete]^2] <> " samples. Subplot (a) " <> DateString["Time"];
ProdTBplotlist = ConstantArray[{0.0, 0.0, 0.0},
  {Length[enDiscrete], Length[enDiscrete]};
For[ii = 1, ii ≤ Length[enDiscrete], ii++,
  For[jj = 1, jj ≤ Length[enDiscrete], jj++,
    ProdTBplotlist[[ii, jj]] = {enDiscrete[[ii]], enDiscrete[[jj]],
      Abs[ProdTBpluslist[[ii, jj, 3]]^2 + Abs[ProdTBminuslist[[ii, jj, 3]]]^2};
  ];
];
ProdTBplotlistfiltered = Select[Flatten[ProdTBplotlist, 1], #[[3]] < 1000 &;
jet[u_?NumericQ] :=
  Blend[{0, RGBColor[0, 0, 9/16]}, {1/9, Blue}, {23/63, Cyan}, {13/21, Yellow},
    {47/63, Orange}, {55/63, Red}, {1, RGBColor[1/2, 0, 0]}], u /; 0 ≤ u ≤ 1;
ProdTBPlot = ListDensityPlot[{#[[1]], #[[2]], Log10[10^-6 + #[[3]]]} &/@ Flatten[
  ProdTBplotlist, 1], PlotRange → {{-2, 2}, {-2, 2}, {-6, 0}}, ColorFunction → jet,
  Epilog → {AbsoluteDashing[{6, 6}], Gray, Line[{wplus, 0}, {0, wplus}],
    Line[{-wplus, 0}, {0, -wplus}]}], ImagePadding → None, Frame → False];
(* Save the figure *)
img =
  Rasterize[ProdTBPlot, ImageSize → 72 * 3, RasterSize → 3 * 600, Background → None];
Export["./fig09/fig09_FreeToBound_prodFunc.png", img, ImageResolution → 600];
Print[img];

(* Create the data for subplot (b) *)
(* We create an interpolating functions to speed up integrations. *)
ProdTBplusInterp = ListInterpolation[ProdTBpluslist[;;, ;;, 3],
  {{Min[enDiscrete], Max[enDiscrete]}, {Min[enDiscrete], Max[enDiscrete]}}];
ProdTBminusInterp = ListInterpolation[ProdTBminuslist[;;, ;;, 3],
  {{Min[enDiscrete], Max[enDiscrete]}, {Min[enDiscrete], Max[enDiscrete]}}];
(* Print[DensityPlot[Log10[10^-6 + Abs[ProdTBplusInterp[x, y]]^2 +
  Abs[ProdTBminusInterp[x, y]]^2], {x, -2, 2}, {y, -2, 2}, PlotRange → {-6, 0},
  ColorFunction → jet, BoundaryStyle → {Thick, Gray}, PlotPoints → 100]; *)
xc = 0; s = 12;
kList = Table[k, {k, π/6, 5 * π/6, π/150}];
resultList = ConstantArray[{0.0, 0.0, 0.0}, Length[kList]];
dum = TimeUsed[];
temp = PrintTemporary["Starting evaluation... " <> DateString["Time"]];
For[i = 1, i ≤ Length[kList], i++,
  ProdTBManual[g_, η_, wpm_, pb_, wk1_, wk2_] = ProdTBplusInterp[wk1, wk2];
  i1 = NIntegrate[Abs[FreeToBoundTB[p, wplus, 0, g, η, xc, s, kList[[i]]]]^2,
    {p, -ArcCos[ $\frac{4 - wplus}{-2 J}$ ], 0}, PrecisionGoal → 2, MaxRecursion → 2000];
  ProdTBManual[g_, η_, wpm_, pb_, wk1_, wk2_] = ProdTBminusInterp[wk1, wk2];
  i2 = NIntegrate[Abs[FreeToBoundTB[p, -wplus, 0, g, η, xc, s, kList[[i]]]]^2,
    {p, -π, -ArcCos[ $\frac{-4 + wplus}{-2 J}$ ]}, PrecisionGoal → 2, MaxRecursion → 2000];
  resultList[[i]] = {kList[[i]], i1, i2};
Export["./fig09/fig09_FreeToBound_integrals_g" <>
  ToString[IntegerPart[10 * gp]] <> ".tsv", N[resultList]];
NotebookDelete[temp];
temp = PrintTemporary[
  "Subplot (b): " <> ToString[TimeUsed[] - dum] <> " seconds for i=" <>
  ToString[i] <> " of " <> ToString[Length[kList]] <> ". Total time estimate " <>

```

```

ToString[(TimeUsed[] - dum) / i * Length[kList]] <> " sec.";
];
Print[ToString[TimeUsed[] - dum] <> " seconds total for " <>
ToString[Length[kList]] <> " samples. " <> DateString["Time"]];
Print[ListPlot[({#[[1]], #[[2]] + #[[3]]}) & /@ resultList,
PlotRange -> {{0,  $\pi$ }, {0,  $6 * 10^{-4}$ }}, Joined -> True, InterpolationOrder -> 2]]
];

```

434.701 seconds total for 6561 samples. Subplot (a) 00:43:33

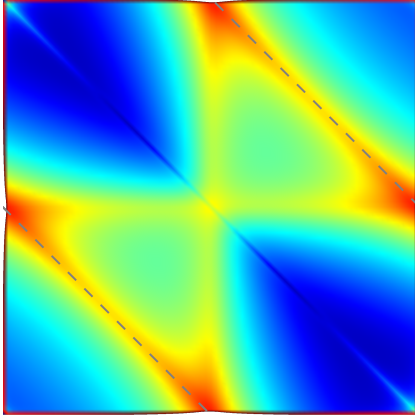

8127.69 seconds total for 101 samples. 02:58:40

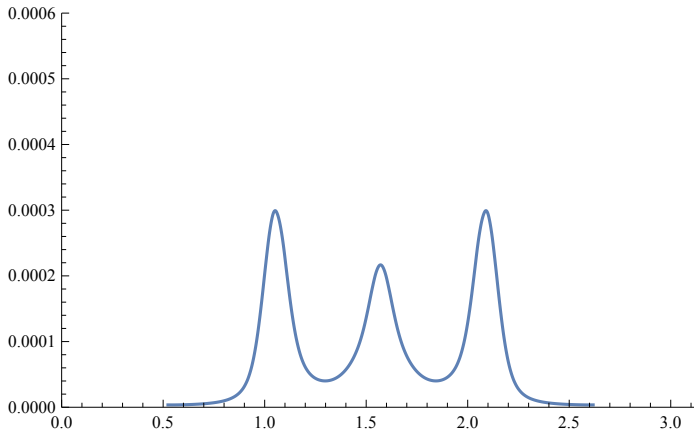

**Fig 10**

This block visualizes (51) in the p1-p2 plane.

```

Block[{ $\eta$ , en,  $\Omega$ , g, J, order, BTBlist, BTBlistfiltered, xc, s, k0, kDiscrete,
TwoPhotonTBList, dum, plotContour, contourPoints, jet, plotInt, img, maxNorm},
(* BTB is the B-function for Tight Binding Lattice *)
 $\eta = 10^{-6}$ ;
en = 2 * (-2 Cos[2  $\pi$  / 5]) +  $i \eta$  // N;
 $\Omega = 0$ ;
g = 0.5 /  $\sqrt{2 \pi}$  // N;
J = 1;
order = 0;
BTBlist = Table[{ $\Delta E_k$ ,  $\Delta E_p$ , Abs[BTB[en,  $\Omega$ , g, order,  $\Delta E_k$ ,  $\Delta E_p$ ]]2},
{ $\Delta E_k$ , Max[-2 - Re[en] / 2, -2 + Re[en] / 2], Min[2 - Re[en] / 2, 2 + Re[en] / 2], 0.01},
{ $\Delta E_p$ , Max[-2 - Re[en] / 2, -2 + Re[en] / 2], Min[2 - Re[en] / 2, 2 + Re[en] / 2], 0.01}];

```

```

BTBlistfiltered = Select[Flatten[BTBlist, 1], #[[3]] < 1000 &];
Print[ListPlot3D[BTBlistfiltered, PlotRange → All]];

(* Create the non-uniform mesh used in visualizations *)
g =  $\frac{0.5}{\sqrt{2\pi}}$ ; xc = 70; s = 12; k0 = 2  $\pi$  / 5;  $\Omega$  = 0;
kDiscrete = Table[{r * Cos[ $\theta$ ], r * Sin[ $\theta$ ]},
  {r,  $\sqrt{2}$  k0 - 5 / s,  $\sqrt{2}$  k0 + 5 / s,  $\frac{1}{20} * 10 / s$ }, { $\theta$ , 0, 2  $\pi$ ,  $\frac{2\pi}{360}$ ]];
AppendTo[kDiscrete, Table[{p1, p2}, {p1, - $\pi$ ,  $\pi$ ,  $\pi / 10$ }, {p2, - $\pi$ ,  $\pi$ ,  $\pi / 10$ }}];
kDiscrete = Partition[Flatten[kDiscrete], 2] // N;
Print[ListPlot[kDiscrete, PlotRange → All]];

(* Create the data by integration defined in FreeToFreeTB function *)
TwoPhotonTBList = ConstantArray[{0.0, 0.0, 0.0}, Length[kDiscrete]];
dum = TimeUsed[];
For[ii = 1, ii ≤ Length[kDiscrete], ii++,
  TwoPhotonTBList[[ii]] = {kDiscrete[[ii, 1]], kDiscrete[[ii, 2]],
    FreeToFreeTB[kDiscrete[[ii, 1]], kDiscrete[[ii, 2]],  $\Omega$ , g, xc, s, k0]};
];
Print[ToString[TimeUsed[] - dum] <>
  " seconds for " <> ToString[Length[kDiscrete]] <> " points."];

(* Create the contour data*)
plotContour = ContourPlot[-2 Cos[k1 *  $\pi$ ] - 2 Cos[k2 *  $\pi$ ] == -4 * Cos[k0], {k1, -1, 1},
  {k2, -1, 1}, ContourStyle → {Black, Dashed}, PlotRangePadding → None];
contourPoints = Cases[Normal@plotContour, Line[pts_, ___], Infinity];

(* Colorfunction definition from *)
(* http://stackoverflow.com/questions/5753508/custom-colorfunction-colordata-in-arrayplot-and-similar-functions/9321152#9321152 *)
jet[u_?NumericQ] := Blend[{0, RGBColor[0, 0, 9 / 16]}, {1 / 9, Blue},
  {23 / 63, Cyan}, {13 / 21, Yellow}, {47 / 63, Orange},
  {55 / 63, Red}, {1, RGBColor[1 / 2, 0, 0]}, u] /; 0 ≤ u ≤ 1;
maxNorm = Max[Abs[#[[3]]]^2] & /@ TwoPhotonTBList;
(* Create the log colored plot*)
plotInt = ListDensityPlot[
  ({#[[1]] /  $\pi$ , #[[2]] /  $\pi$ , Log10[10-7 + Abs[#[[3]]]^2 / maxNorm]} & /@ TwoPhotonTBList,
  PlotRange → {{-1, 1}, {-1, 1}, {-7, 0}}, ColorFunction → jet,
  InterpolationOrder → 2, Mesh → None, PlotRangePadding → None,
  Epilog → {AbsoluteDashing[{6, 6}], Gray, contourPoints}];
img = Rasterize[Show[plotInt, Frame → False, ImagePadding → None],
  ImageSize → 72 * 3, RasterSize → 3 * 600, Background → None];
Print[img];
Export["./fig10/fig10_FigFreeToFree_Mathematica.png", img, ImageResolution → 600];
];

```

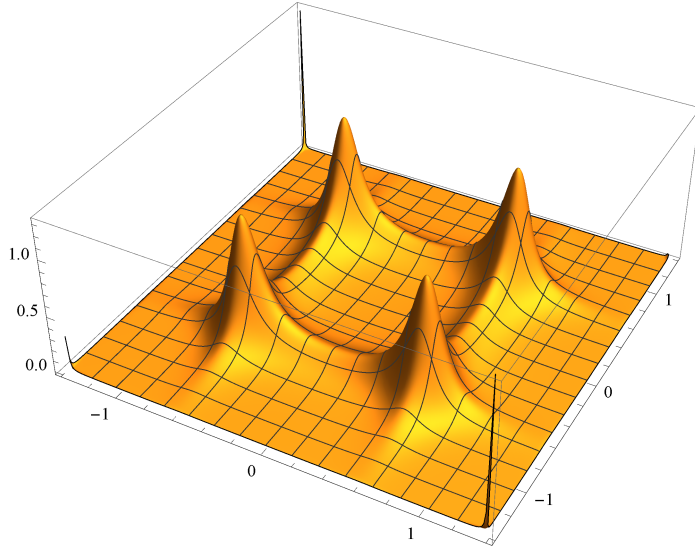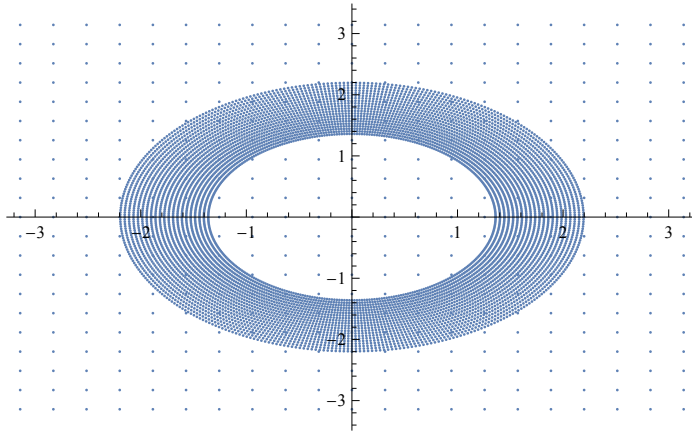

209.049 seconds for 8022 points.

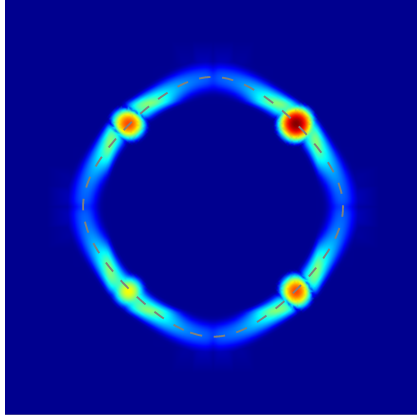

## Comparison with Ref [46] arXiv:0907.2776 (Shi2009)

These calculations aim to reproduce Figs 3a and 3b in Shi2009 to check our implementation, and then to compare the Shi2009 expressions with Fig 7 parameters.

To reproduce Figs 3a&3b, a number of parameters need to be calculated.

In order to calculate  $E_s$  we need to find the zeros of the expression  $\mathbf{z} - \Omega - \frac{g\mathbf{p}^2}{2\pi} \mathbf{Int}[\mathbf{z} - \omega\mathbf{0}]$ . Here  $g\mathbf{p}$  is the same as the  $V$  parameter in Shi2009, also  $\frac{g\mathbf{p}^2}{2\pi} \mathbf{Int}[\mathbf{z} - \omega\mathbf{0}]$  refers to  $\Sigma(z)$  in Shi2009 notation. When  $z$  coincides with the real axis, we can get a closed form

$$\text{formula for } \Sigma(\omega) = \frac{V^2}{2\pi} \int_{-\pi}^{\pi} dk \frac{1}{\omega - \omega_0 + 2J \cos k} = V^2 \begin{cases} \frac{1}{\sqrt{(\omega - \omega_0)^2 - 4J^2}} & \omega - \omega_0 > 2J \\ \frac{-i}{\sqrt{4J^2 - (\omega - \omega_0)^2}} & -2J < \omega - \omega_0 < 2J \\ \frac{-1}{\sqrt{(\omega - \omega_0)^2 - 4J^2}} & \omega - \omega_0 < -2J \end{cases}$$

by using the results from App A of the manuscript.

Below we write a polynomial equation for  $\mathbf{z} - \Omega - \frac{gp^2}{2\pi} \text{Int}[\mathbf{z} - \omega 0] = 0$ , solve it, and weed out the unphysical zeros by testing to make sure the equation  $\mathbf{z} - \Omega - \frac{gp^2}{2\pi} \text{Int}[\mathbf{z} - \omega 0] = 0$  holds. At the output we show the bound state energies and dispersion for the parameters in Figs 3a & 3b.

Fig 3a refers to bound to bound scattering for  $\Omega = 2.5$  and Fig 3b for  $\Omega = 5$ . In both cases  $\omega_0 = 4$ ,  $J = V = 1$ . Fig 3a is for scattering from  $E_1$  bound state ( $s=1$ ), Fig 3b is for scattering from  $E_2$  bound state ( $s=2$ ).

The index of the bound state,  $s$ , is stored in **sList**.

$G^+$  and  $J^+$  functions are given by **Gp[z]** and **Jp[z1, z2]**.

$E_s$  and  $E_{\bar{s}}$  are given by **Es** and **Esb** variables.

$Z_s$  and  $Z_{\bar{s}}$  are given by **Zs** and **Zsb** variables.

$E^{(s)}$  is given by **Espar** variable.

You can see below that we were able to replicate Fig 3a and 3b of Shi2009.

In order to compare Shi2009 results with results from Fig 7d of the manuscript, we run Shi2009 calculations with  $\Omega = \omega_0$ , which corresponds to the  $\Omega = 0$  case in the manuscript, with a shift in zero-level energy by  $\omega_0$ . Fig 7d is plotted as a function of  $k$ , we re-plot it as a function of shifted energy to compare with Shi2009. The two approaches agree very well with one another.

```
Block[{fptest, fpoly, gp, w0, J, OmegaList, resultList,
  soln, OmegaList, sList, plotList, Omega, s, Gp, Jp, Es, Esb, Zs, Zsb,
  en0List, RListFig3, TListFig3, RpTListFig3, Espar, As, R2list},

  fptest[z_, w0_, Omega_, gp_] := z - Omega - \frac{gp^2}{2\pi} \text{Int}[z - w0];
  fpoly[z_, w0_, Omega_, gp_] := ((z - w0)^2 - 4) (z - Omega)^2 - gp^4;
  (* Calculate Es and plot*)
  gp = 1; w0 = 4; J = 1;
  OmegaList = Table[Omega, {Omega, {w0 - 5.0, w0 + 5.0, 0.05}}];
  resultList = {};
  For[i = 1, i <= Length[OmegaList], i++,
    soln = Cases[z /. NSolve[fpoly[z, w0, OmegaList[[i]], gp] == 0], _Real];
    For[j = 1, j <= Length[soln], j++,
      If[Abs[fptest[soln[[j]], w0, OmegaList[[i]], gp]] < 10^-5,
        AppendTo[resultList, {OmegaList[[i]], soln[[j]]}];
      ];
    ];
  Print[ListPlot[{Select[resultList, #[[2]] > w0 &], Select[resultList, #[[2]] < w0 &]},
    Joined -> True, PlotStyle -> {Blue, Black}, AxesLabel -> {"Omega", "Es"},
    Epilog -> {Dashed, Red, Line[{{w0 + 5, w0 + 5}, {w0 - 5, w0 - 5}}],
      Red, Line[{{w0, w0 + 5}, {w0, w0 - 5}}], PointSize[Large], Point[
        Select[resultList, #[[1]] == 2.5 &]], Point[Select[resultList, #[[1]] == 5.0 &]]},
    Ticks -> {Range[w0 - 5, w0 + 5, 1], Range[w0 - 5, w0 + 5, 1]},
    PlotLabel -> "E1 (black) and E2 (blue) for w0=" <> ToString[w0] <>
      ", V=" <> ToString[gp] <> ", J=" <> ToString[J], ImageSize -> 72 * 4];
  Print[Select[resultList, #[[1]] == 2.5 &];
  Print[Select[resultList, #[[1]] == 5.0 &];

  (* Calculate the integrals and get reflection coefficient for three cases *)
  (* The first two cases give Shi2009 Fig 3a, 3b. Last case gives Fig 7d *)
```

```

ΩList = {2.5, 5, ω0};
sList = {1, 2, 1};
plotList = {};
For[i = 1, i ≤ Length[ΩList], i++,
  Ω = ΩList[[i]];
  s = sList[[i]];

  Gp[z_?NumericQ] :=  $\left(z - \Omega - \frac{gp^2}{2\pi} \text{Int}[z - \omega 0]\right)^{-1}$ ;

  Jp[z1_?NumericQ, z2_?NumericQ] :=  $\frac{1}{\pi} \frac{Gp[z1]}{(z2 - z1)}$ ;

  Es = Sort[Select[resultList, #[[1]] == Ω &][[;;, 2]], Smaller];
  Esb = Sort[Select[resultList, #[[1]] == Ω &][[;;, 2]], Greater];

  Zs =  $\left\{ \left( 1 + \frac{gp^2}{2\pi} \text{NIntegrate} \left[ \frac{1}{(Es[[1]] - (\omega 0 - 2 J \cos[k]))^2}, \{k, -\pi, \pi\} \right] \right)^{-1}, \right.$ 
     $\left. \left( 1 + \frac{gp^2}{2\pi} \text{NIntegrate} \left[ \frac{1}{(Es[[2]] - (\omega 0 - 2 J \cos[k]))^2}, \{k, -\pi, \pi\} \right] \right)^{-1} \right\}$ ;

  Zsb = {Zs[[2]], Zs[[1]]};
  en0List = Table[en, {en, ω0 - 2 J, ω0 + 2 J, J / 50}];
  RListFig3 = ConstantArray[{0.0, 0.0}, Length[en0List]];
  TListFig3 = ConstantArray[{0.0, 0.0}, Length[en0List]];
  RpTListFig3 = ConstantArray[{0.0, 0.0}, Length[en0List]]; (*R plus T list *)

  For[j = 1, j ≤ Length[en0List], j++,
    Espar = Es[[s]] + en0List[[j]];
    As =  $\frac{Zsb[[s]] (Esb[[s]] - Es[[s]]) Gp[Espar - Esb[[s]]]}{Espar - Esb[[s]] - en0List[[j]]}$  +
       $\text{NIntegrate} \left[ Jp[Espar - enp + i * 10^{-6}, en0List[[j]]] (enp - Es[[s]]) \text{Im}[Gp[enp]], \right.$ 
         $\{enp, \omega 0 - 2 J, \omega 0 + 2 J\}, \text{PrecisionGoal} \rightarrow 5, \text{MaxRecursion} \rightarrow 1000,$ 
         $\text{Method} \rightarrow \{\text{GlobalAdaptive}, \text{MaxErrorIncreases} \rightarrow 10000\} \Big]$ ;

    RListFig3[[j]] =  $\left\{ en0List[[j]], \text{Abs} \left[ \frac{i * gp^2 * Gp[en0List[[j]]]}{2 * J * \text{Abs} \left[ \text{Sin} \left[ \text{ArcCos} \left[ \frac{en0List[[j]] - \omega 0}{-2 J} \right] \right] \right]} \right. \right.$ 
       $\left. \left. \frac{Zs[[s]] * Gp[en0List[[j]]] + As}{Zs[[s]] * Gp[en0List[[j]]] - As} \right]^2 \right\}$ ;

    TListFig3[[j]] =  $\left\{ en0List[[j]], \text{Abs} \left[ 1 + \frac{i * gp^2 * Gp[en0List[[j]]]}{2 * J * \text{Abs} \left[ \text{Sin} \left[ \text{ArcCos} \left[ \frac{en0List[[j]] - \omega 0}{-2 J} \right] \right] \right]} \right] \right.$ 
       $\left. \left. \frac{Zs[[s]] * Gp[en0List[[j]]] + As}{Zs[[s]] * Gp[en0List[[j]]] - As} \right]^2 \right\}$ ;

    RpTListFig3[[j]] = {en0List[[j]], RListFig3[[j, 2]] + TListFig3[[j, 2]]};
  ];

  RListFig3 = Cases[RListFig3, {_?NumericQ, _?NumericQ}];
  TListFig3 = Cases[TListFig3, {_?NumericQ, _?NumericQ}];
  RpTListFig3 = Cases[RpTListFig3, {_?NumericQ, _?NumericQ}];
  AppendTo[plotList, ListPlot[{RListFig3, TListFig3, RpTListFig3},
    PlotStyle → {{Dotted, Blue}, {Dashed, Red}, {Dashing[{}], Green}},
    Joined → True, Frame → True, ImageSize → 72 * 3]];
];
Print["Reproduction of Shi2009a Fig 3a & 3b"];

```



```

Print[GraphicsRow[plotList[[1 ;; 2]]]];
Print["Comparison to Fig 7d"];
(* The k-index is converted to energy and shifted by w0 to compare with Fig 7d *)
R2list = ({-2 J * Cos[#[[2]]] + w0, Abs[#[[3]]]^2}) & /@ ToExpression[
  Import["./fig07/integrals_r2_g" <> ToString[IntegerPart[10 * gp]] <> ".tsv"]];
Print[Show[plotList[[3]], ListPlot[R2list,
  PlotMarkers -> Graphics@{Disk[{0, 0}, Scaled@0.02]}]]];
];

```

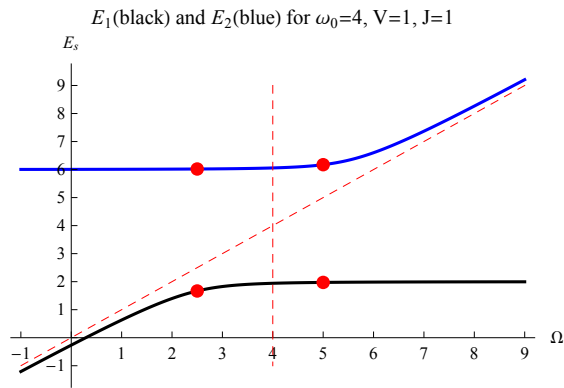

```
{{2.5, 1.66721}, {2.5, 6.02008}}
```

```
{{5., 1.9729}, {5., 6.17387}}
```

Reproduction of Shi2009a Fig 3a & 3b

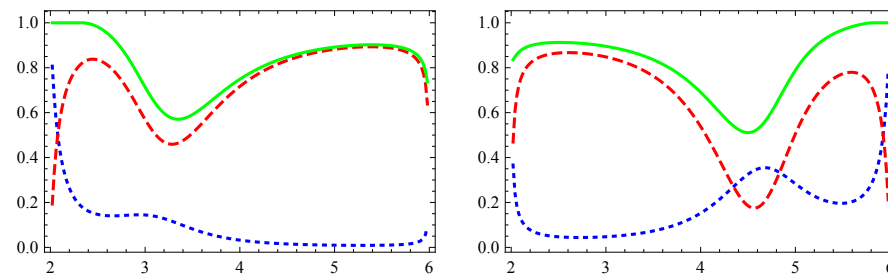

Comparison to Fig 7d

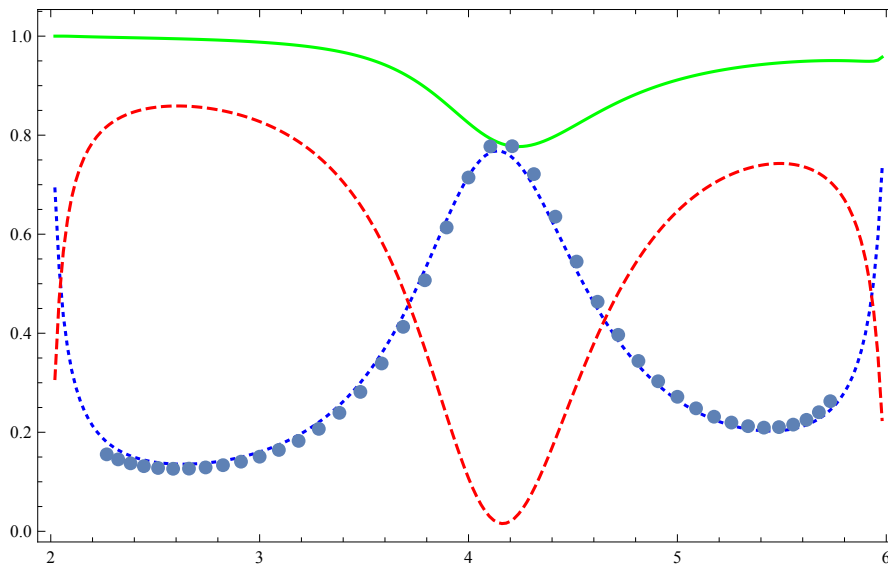

Supplement: Supplementary file 1 [file figureCalculations.pdf]
